# Supplementary material for: Hole in one: Pathways to deterministic single-acceptor incorporation in Si(100)-2$\times$1
Source: arXiv:2108.10805 source file (2021-08-24)
Supplement: Supplementary file 1 [file sm.tex]

% Supplementary information starts here
\clearpage
\widetext
\begin{center}
\textbf{\large Supplementary information: Pathways to deterministic atomic-precision single acceptor incorporation on Si(100)2$\times$1}
\end{center}

% Reset counters and add an S prefix on equation and figure numbers
\setcounter{section}{0}
\setcounter{page}{1}
\makeatletter

% This is Andrew's ongoing rewrite of the SM.
%%%%%%%%%%%%%%%%%%%%%%%%%%%%%%%%%%%%%%%%%%%%%%%%%%%%%%%%%%%%%%%%%%%%%%%%%%%%%%%%%%%%%%%%%%%%%%%%
\section*{Contents}

The Supplemental Materials elaborate on details of some of the central results in the main body of the paper.
\begin{itemize}
    \item Appendix A describes...
\end{itemize}

\section*{Appendix A: }
\setcounter{equation}{0}
\setcounter{figure}{0}

\label{app:expt_details}
